# Supplementary material for: Collapsing Bandits and Their Application to Public Health Interventions
Source: arXiv:2007.04432 source file (2020-07-05)
Supplement: Supplementary file 1 [file appendix_self_contained.tex]

\documentclass{article}

% if you need to pass options to natbib, use, e.g.:
%     \PassOptionsToPackage{numbers, compress}{natbib}
% before loading neurips_2020

% ready for submission
% \usepackage{neurips_2020}

% to compile a preprint version, e.g., for submission to arXiv, add add the
% [preprint] option:
%     \usepackage[preprint]{neurips_2020}

% to compile a camera-ready version, add the [final] option, e.g.:
%     \usepackage[final]{neurips_2020}

% to avoid loading the natbib package, add option nonatbib:
\PassOptionsToPackage{numbers}{natbib}
\usepackage{neurips_2020}

\usepackage[utf8]{inputenc} % allow utf-8 input
\usepackage[T1]{fontenc}    % use 8-bit T1 fonts
\usepackage{hyperref}       % hyperlinks
\usepackage{url}            % simple URL typesetting
\usepackage{booktabs}       % professional-quality tables
\usepackage{amsfonts}       % blackboard math symbols
\usepackage{nicefrac}       % compact symbols for 1/2, etc.
\usepackage{microtype}      % microtypography
\usepackage[pdftex]{graphicx}

\usepackage{enumitem}
\usepackage{amsmath, amssymb}
\usepackage{bbm}
\usepackage[ruled,vlined]{algorithm2e}
\usepackage{algorithmic}
\usepackage{amsthm}
\usepackage{subfig}

\usepackage{tikz}
\usetikzlibrary{automata}
\usetikzlibrary{calc, automata, chains, arrows.meta}
\usetikzlibrary{chains,scopes}
\usetikzlibrary{positioning}

\usepackage{enumitem}
\usepackage{amsmath, amssymb}
\usepackage{bbm}
\usepackage[ruled,vlined]{algorithm2e}
\usepackage{algorithmic}
\usepackage[subtle]{savetrees}
% \linespread{0.97}
\usepackage{amsthm}
\usepackage{subfig}
\usepackage{mathtools}

\title{Collapsing/Monitoring Bandits: Restless Bandits with State Dependent Resets \\ Online Appendix
}

% The \author macro works with any number of authors. There are two commands
% used to separate the names and addresses of multiple authors: \And and \AND.
%
% Using \And between authors leaves it to LaTeX to determine where to break the
% lines. Using \AND forces a line break at that point. So, if LaTeX puts 3 of 4
% authors names on the first line, and the last on the second line, try using
% \AND instead of \And before the third author name.

\author{%
  Jackson A. Killian\thanks{equal contribution.} \\
  School of Engineering and Applied Sciences\\
  Harvard University\\
  Cambridge, MA, 02138 \\
  \texttt{jkillian@g.harvard.edu} \\
%   examples of more authors
   \And
   Aditya Mate$^*$ \\
  School of Engineering and Applied Sciences\\
  Harvard University\\
  Cambridge, MA, 02138 \\
  \texttt{aditya_mate@g.harvard.edu} \\
  \And
  Haifeng Xu \\
  Computer Science\\
  University f Virginia\\
  Charlottesville, Virginia 22904 \\
  \texttt{hx4ad@virginia.edu} \\
  \And
  Andrew Perrault \\
  School of Engineering and Applied Sciences\\
  Harvard University\\
  Cambridge, MA, 02138 \\
  \texttt{aperrault@g.harvard.edu} \\
  \And
  Milind Tambe \\
  School of Engineering and Applied Sciences\\
  Harvard University\\
  Cambridge, MA, 02138 \\
  \texttt{milind_tambe@harvard.edu} \\
}

\begin{document}

\maketitle

\input{appendix}

\end{document}
